# Supplementary material for: Information Processing in Hybrid Photonic Electrical Reservoir Computing
Source: arXiv:2404.01479 source file (2024-04-01)
Supplement: Supplementary file 1 [file Supplemenatry_material.pdf]

# Supplementary Material

## 1. HPE-RC device

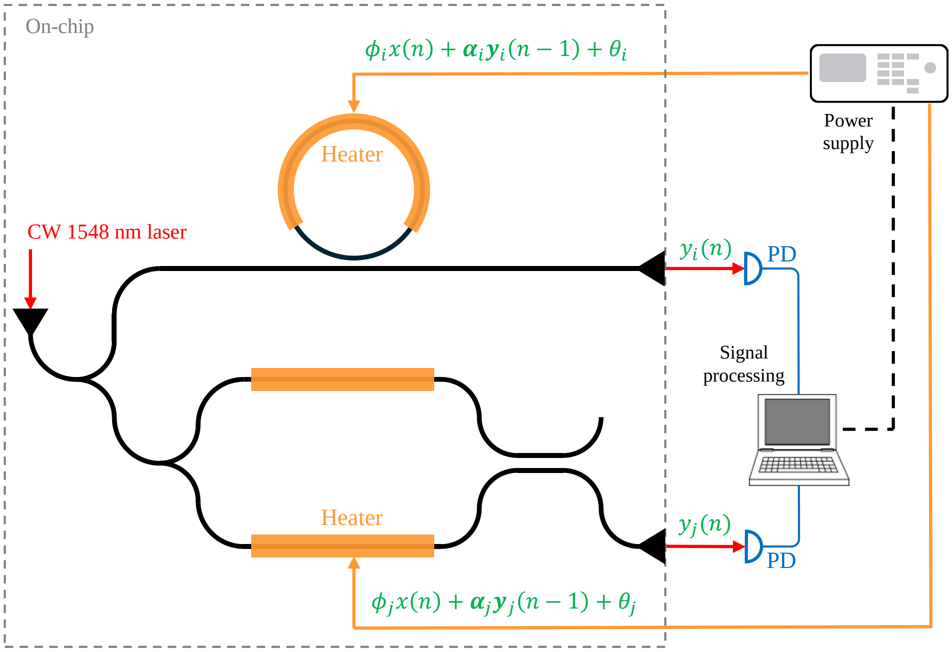


**Fig. S1**. An illustration of the setup for HPE-RC. The grating coupler on the chip is fed by a CW laser at 1548 nm wavelength, which sends the optical power to the MZI and ring resonator. After interacting with each optical device, the lightwave leaves the chip by a grating coupler and is converted to an electrical signal by a photodetector (PD). The signal is processed by a digital computer which sends the input and feedback of the HPE-RC to the metal heaters through a power supply. The metal heaters change the optical index of the cladding silicon dioxide layer and the silicon waveguide, and provide the phase modulation to encode the signal in the optical devices. The digital computer performs the ridge regression for training and then implements the trained weights to perform a specific task. The Ls_mRMR algorithm is also implemented offline on the digital computer.

The setup for HPE-RC is shown in fig. S1. A 500 nm x 220 nm silicon waveguide buried in the silicon oxide carries the optical power in the MZI and ring resonator. The cross-section of the optical mode is shown in fig. S2a. The phase modulation in the HPE-RC is provided by the metal heaters. When voltage $V$ is applied on the heater, the generated heat will change the optical index of the silicon waveguide, Fig. S2a shows the cross-section geometry and the COMSOL simulated temperature distribution of the heater-waveguide structure under $5V$ applied voltage and $12.5\ mA$ measured current in $L = 400\ \mu m$ long TiW heater. Fig. S2b presents the simulation result and fitted curve of average temperature in the waveguide area versus applied voltage, Fig. S2c is the simulation results of effective mode index versus temperature change using thermo-optic coefficient $dn/dT = 1.8 \times 10^{-4}\ 1/K$ [37]. With these simulations, we can directly relate $V$ to the induced phase delay and numerically calculate the output power of the device

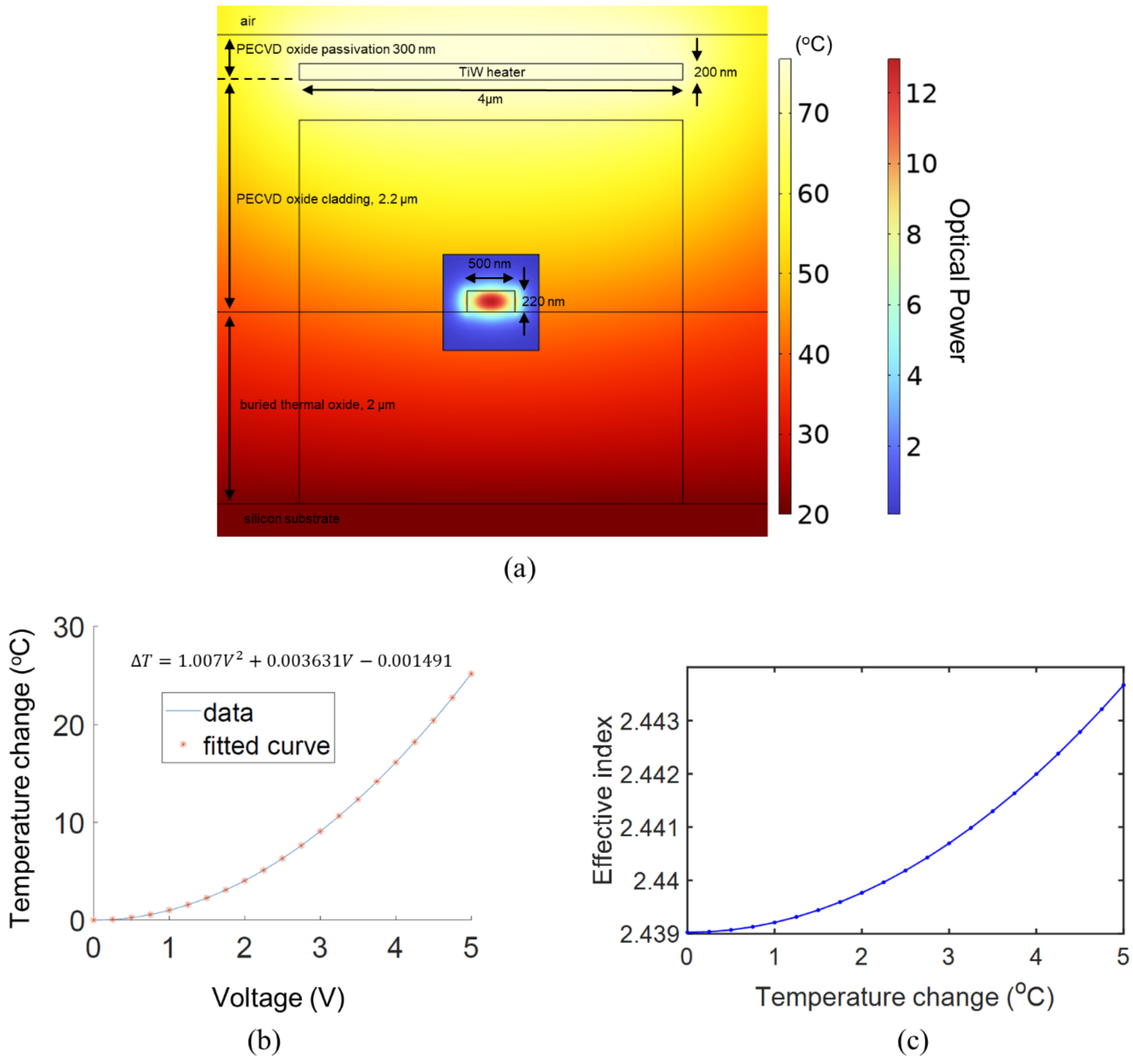


**Fig. S2**. (a) COMSOL simulation of mode in a 500 nm x 220 nm silicon waveguide and the distribution of temperature by a TiW heater. The voltage applied to the heater is 5 V and the measured current is 12.5 A when the length of the heater is 400 µm. (b) Plot of average temperature change in waveguide against voltage applied. The curve can be fitted by a second-order function of voltage which is also shown. (c) the simulation results of effective mode index versus temperature change using thermo-optic coefficient $dn/dT = 1.8 \times 10^{-4}\ 1/K$

The evanescent couplers and splitters are simulated and designed to be 50:50 at 1550 nm wavelength. The MZI is balanced with each arm length being 400 µm. The radius of the loop waveguide used in the ring resonator is 50 µm and the gap between the loop and bus waveguide is 100 nm. The SEM images of the evanescent couplers, splitter, grating coupler and coupling region of the ring is shown in Fig. S3. The transmission spectra of 2 couplers and a waveguide, the MZI and ring resonator is shown in Fig. S4.

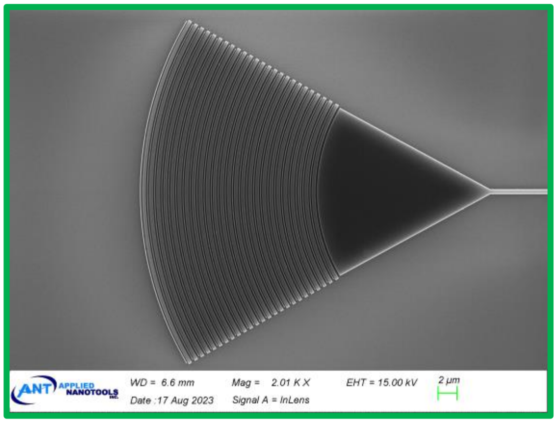


(a)

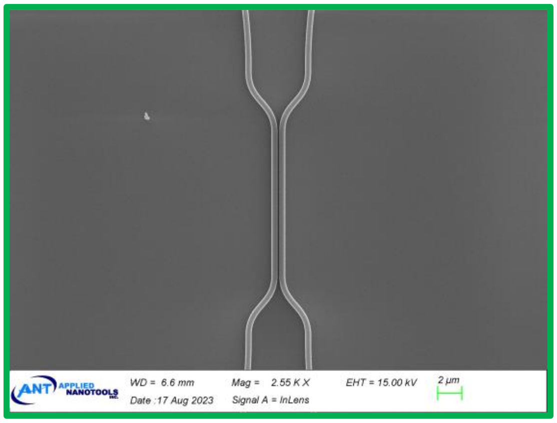


(b)

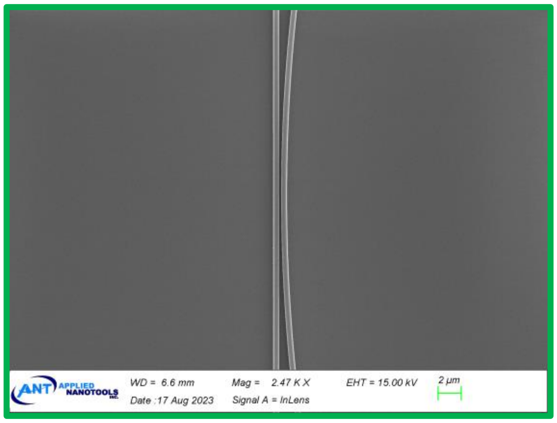


(c)

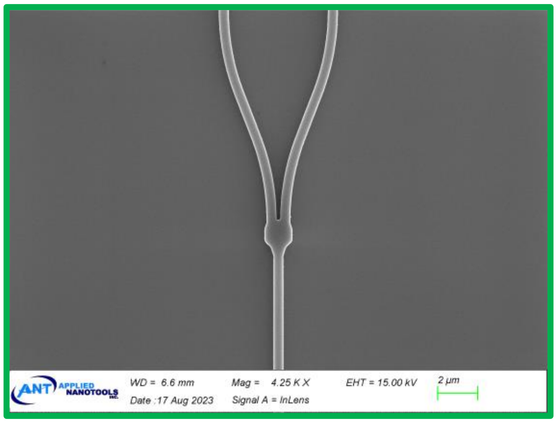


(d)

**Fig. S3**. SEM images of (a) Grating couplers used to send and receive optical power from the chip. (b) 50:50 evanescent couplers used to design the MZI. (c) Coupling region of the ring resonator. (d) 50:50 splitter to distribute optical power on the chip.

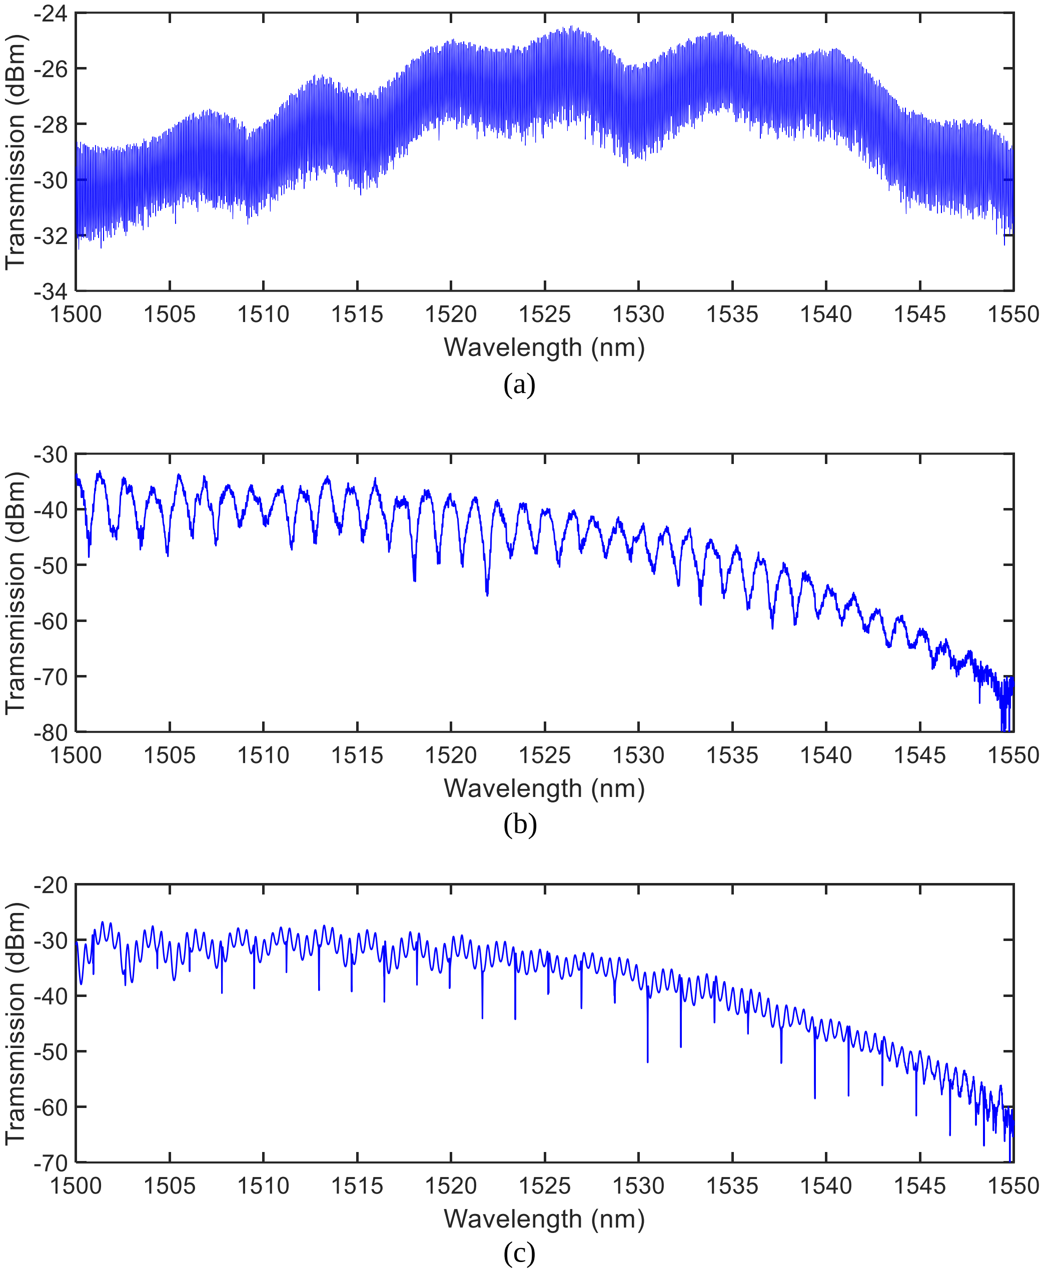


**Fig. S4**. Transmission Spectra of (a) a waveguide 4.3 mm waveguide with 2 couplers at input and output. (b) MZI device (c) ring resonator device.

## 2. Lyapunov Exponent

Let the dynamic function representing the RC be given by:

$$F^n\big(y(l-1)\big) = y(n) = f(\phi x(n) + \boldsymbol{\alpha} \cdot \boldsymbol{y}(n-1) + \theta) = f(\eta(n)) \tag{S1}$$

where $l$ represents the length of the feedback and $y(l-1)$ and is the initial condition of the system and $y(i) = 0 \; \forall \; i < l-1$. The Lyapunov exponent measures how quickly an infinitesimally small distance between two initial close states grows over time:

$$F^n(y(l-1)+\epsilon) - F^n(y(l-1)) \approx \epsilon e^{\lambda n} \tag{S2}$$

$\epsilon$ is a small change in the initial condition that may change the trajectory of the dynamics. The equation can be rearranged to

$$\lambda \approx \frac{1}{n}\log\left(\frac{|F^n(y(l-1)+\epsilon) - F^n(y(l-1))|}{\epsilon}\right) \tag{S3}$$

We take limits on both sides

$$\lambda = \lim_{n\to\infty,\epsilon\to 0}\frac{1}{n}\log\left(\frac{|F^n(y(l-1)+\epsilon) - F^n(y(l-1))|}{\epsilon}\right) \tag{S4}$$

$$\lambda = \lim_{n\to\infty}\frac{1}{n}\log\left|\frac{dF^n}{dy(l-1)}\right| \tag{S5}$$

Using chain rule this can be expressed by

$$\lambda = \lim_{n\to\infty}\frac{1}{n}\log\left(|f'(\eta(n))|.\left|\boldsymbol{\alpha}\cdot\frac{d\boldsymbol{F}^{n-1}}{dy(l-1)}\right|\right) \tag{S6}$$

$\boldsymbol{F}^{n-1}$ is the function vector $[F^{n-1}, F^{n-2}, \dots, F^{n-l}]$. Eq. S6 can be used to recursively calculate the derivative of function $F$ with respect to the initial condition at each time step and results in Algorithm 1 in the main text. Lyapunov exponent for various parameters is shown in fig. S5 and fig. S6.

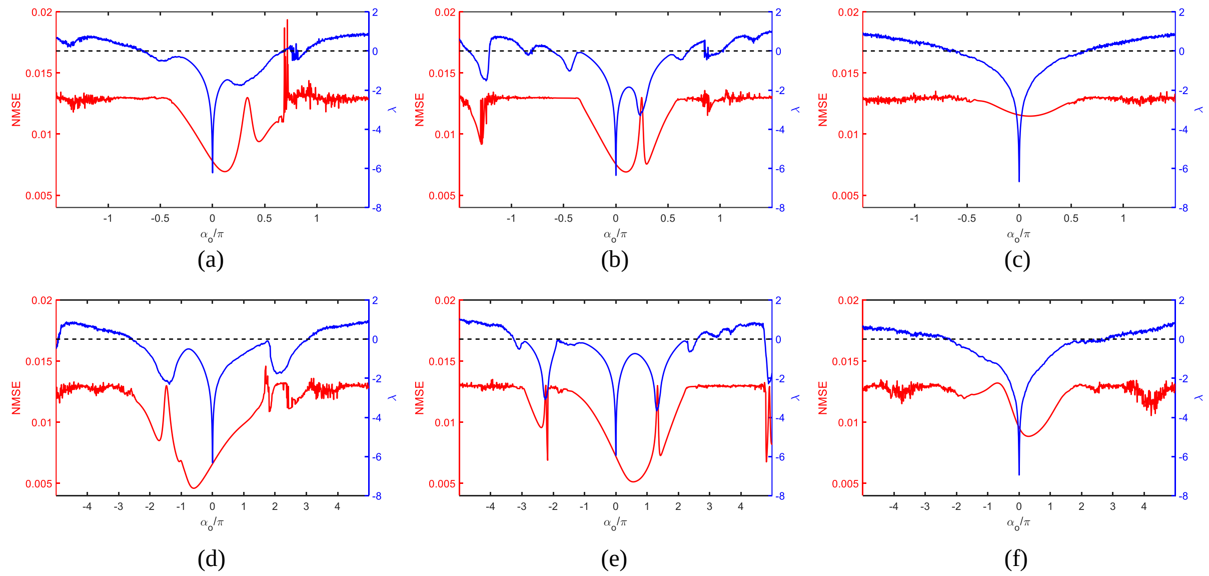


**Fig. S5**. Performance as a single node for NARMA2 task plotted against the Lyapunov exponent. $l = 1$ for this task and $\alpha_o$ is swept for a fixed $\phi$ and $\theta$. MZI: **(a)** $\phi = -0.35\pi, \theta = 0$. **(b)** $\phi = 0.1\pi, \theta = 0.2\pi$. **(c)** $\phi = 1.5\pi, \theta = 0.5\pi$. Ring resonator: **(d)** $\phi = -0.35\pi, \theta = 0$. **(e)** $\phi = 0.1\pi, \theta = 0.2\pi$. **(f)** $\phi = 1.5\pi, \theta = 0.5\pi$.

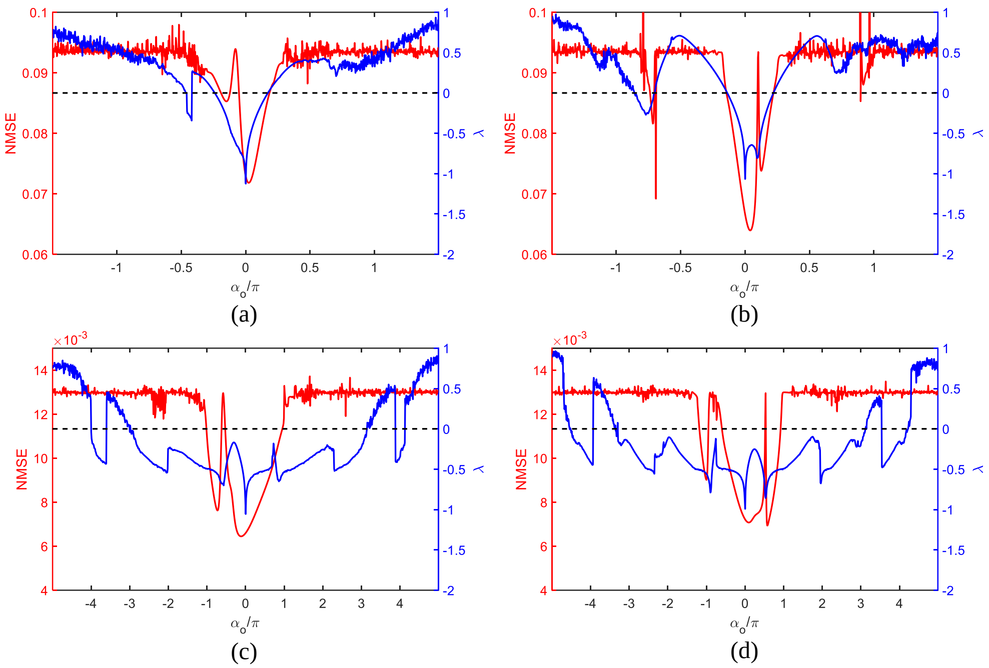


**Fig. S6**. Performance of device as a single node for NARMA10 task plotted against the Lyapunov exponent. $l = 9$ for this task and $\alpha_o$ is swept for a fixed $\phi$ and $\theta$. **(a)** MZI with $\phi = -0.35\pi, \theta = 0$. **(b)** MZI with $\phi = 0.1\pi, \theta = 0.2\pi$. **(a)** Ring Resonator with $\phi = -0.35\pi, \theta = 0$. **(b)** Ring Resonator with $\phi = 0.1\pi, \theta = 0.2\pi$.

## 3. Normalized Mean Square Error (NMSE)

Let the output of $i^{\text{th}}$ node of the reservoir be given by $y_i(n)$ and the task that the reservoir needs to emulate given by $z(n)$. $n$ denotes the time step here and total number of nodes is $K$. The ridge regression trains $K + 1$ weights given by $w_j$ where $0 \le j \le K$. The output of the RC at a given time step $n$ is given by $w_0 + \sum_{i=1}^{K} w_i y_i(n)$. If the total number time steps for which RC performs a task is $N$, the NMSE can be given by the equation

$$\text{NMSE} = \frac{\sum_{n=1}^{N}\left(w_o + \sum_{i=1}^{K} w_i y_i(n) - z(n)\right)^2}{\sum_{n=1}^{N}\left(z(n)\right)^2} \tag{S7}$$
